# Supplementary material for: Optimal Pricing of Internet of Things: A Machine Learning Approach
Source: arXiv:2002.05929 source file (2020-02-14)
Supplement: Supplementary file 1 [file appendix.tex]

\section{Appendix}\label{appendix:appendix}

The appendix, if required, should be placed here.
